# Supplementary material for: What Went Wrong? Explaining Overall Dialogue Quality through Utterance-Level Impacts
Source: arXiv:2111.00572 source file (2021-10-31)
Supplement: Supplementary file 1 [file 10-Appendix.tex]

\appendix
\section{Data Preprocessing and Model Hyperparameters}
\label{sec:params}

\paragraph{AP19}

All utterances in the AP19 dataset were preprocessed by removing all punctuation. All models were trained using the Adam optimizer with a learning rate of 0.00001 and Mean Squared Error loss function. All models had a dropout layer of 0.1 applied to the utterance embeddings. The \textit{ARA-O} and \textit{NARA} models had a hidden dimension of 200. The \textit{ARA-A} had 1 layer with 1 head, hidden dimension 200, and dropout of 0.1 in the Transformer layer.

\paragraph{ConvAI}

All utterances in the ConvAI dataset were preprocessed by converting all symbols to a language representation (e.g. \textbf{\textgreater:(} to 'angry face', \textbf{lol} to 'laughing out loud', and so on) and then removing all remaining punctuation. In addition, multiple sequential utterances by the same speaker in a conversation were concatenated together into a single response.

All models were trained with the Adam optimizer with a learning rate of 0.00001 and Mean Squared Error loss function. All models had a dropout layer applied to the utterance embeddings (\textit{ARA}: 0.2, \textit{Others}: 0.1). The \textit{ARA-O} and \textit{NARA} models had a hidden dimension of 200. The \textit{ARA-A} had 1 layer with 1 head, hidden dimension 100, and dropout of 0.1 in the Transformer layer.
